# Supplementary material for: Not All Parameters Matter: Masking Diffusion Models for Enhancing Generation Ability
Source: arXiv:2505.03097 source file (2025-05-06)
Supplement: Supplementary file 1 [file X_suppl.tex]

\clearpage
\setcounter{page}{1}
\maketitlesupplementary
\appendix

\section{Additional Ablation Studies}
We present the results of different reward models in Table~\ref{tab:t2icompbench-abla}. Overall, the impact of excluding a specific reward model (e.g., HPSv2~\cite{wu2023human} or ImageReward~\cite{xu2024imagereward}) demonstrates that while these individual models positively contribute to specific tasks, they are not the sole determining factors, and their combination maximizes performance improvement. This further validates the importance of leveraging multiple reward signals comprehensively, enabling the capture of more holistic semantic features for semantic binding tasks.
\begin{table}[htbp]
\vspace{-0.1cm}
  \centering
  \caption{Ablation study on the impact of different reward models on T2I-CompBench, with the best results in \textbf{bold}.}
  \vspace{-0.3cm}
  \resizebox{0.94\linewidth}{!}{
    \begin{tabular}{c|ccc}
    \toprule
    \multirow{2}[4]{*}{Method} & \multicolumn{3}{c}{BLIP-VQA} \\
\cmidrule{2-4}     & Color ($\uparrow$) & Texture ($\uparrow$) & Shape ($\uparrow$) \\
    \midrule\midrule
    SD 1.5 \cite{rombach2022high} & 0.3750  & 0.4159  & 0.3742  \\
    % \midrule
    % SD 2.0 \cite{rombach2022high} &50& 0.5056  & 0.4922  & 0.4221  \\
    % \midrule
    % DALL-E 2 &50& 0.5750  & 0.6374  & 0.5464  \\
    % \midrule
    % SDXL  &50& 0.6369  & 0.5637  & 0.5480  \\
    % \midrule
    % PlayG-v2 &50& 0.6208  & 0.6125  & 0.5087  \\
    \midrule
    % w/o hpsv2 &15& 0.5144  & 0.5154  & 0.4447  \\
    % \midrule
    w/o HPSv2~\cite{wu2023human} & 0.4530  & 0.4871  & 0.4202  \\
    % \midrule
    w/o ImageReward~\cite{xu2024imagereward} & 0.4502  & \textbf{0.4949}  & 0.4254  \\
    \midrule
    MaskUNet  & \textbf{0.4958}  & 0.4938  & \textbf{0.4529}  \\
    % \midrule
    % SynGen+MaskUNet &15& 0.\textbf{6989}  & \textbf{0.6209}  & \textbf{0.4644}  \\
    \bottomrule
    \end{tabular}%
    }
  \label{tab:t2icompbench-abla}%
\end{table}%

\section{Additional Results}

\begin{figure}[t]
  \centering
  % \fbox{\rule{0pt}{2in} \rule{0.9\linewidth}{0pt}}
   \includegraphics[width=1.\linewidth]{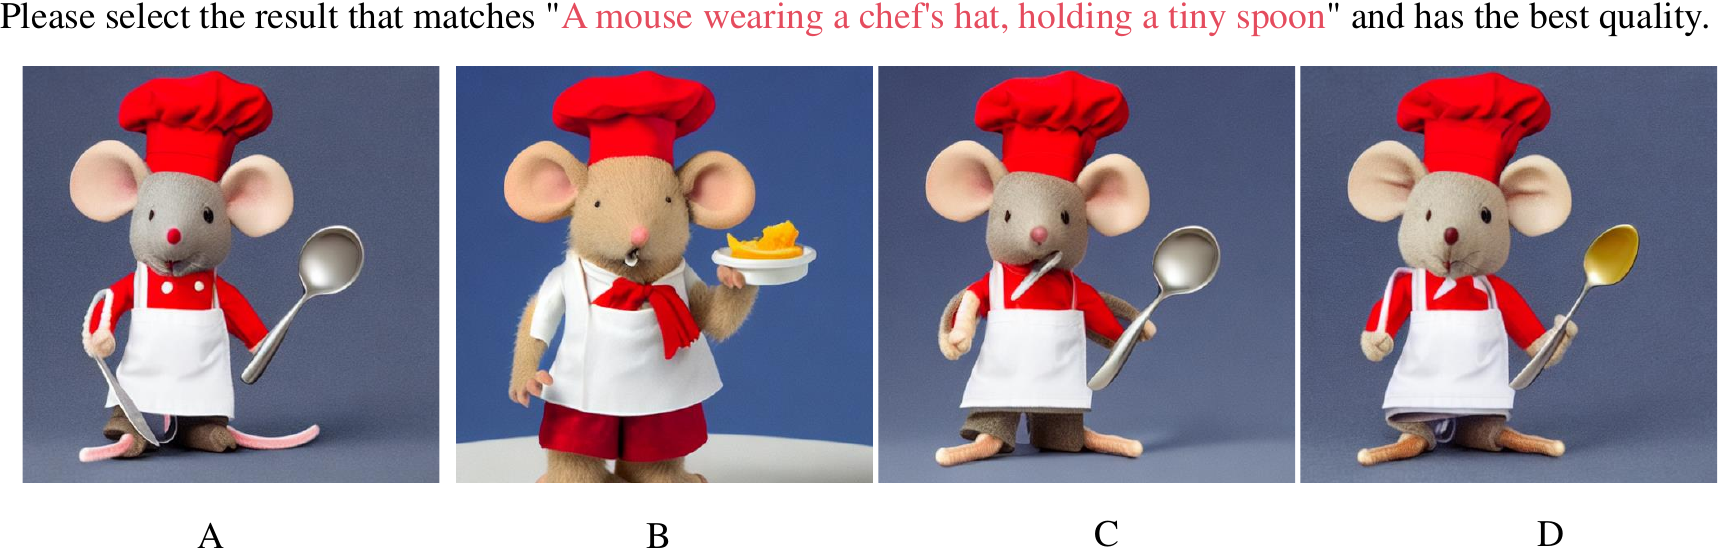}
   \vspace{-0.3cm}
   \caption{An example of the user study.}
   \label{fig:user_exam}
% \vspace{-0.5cm}
\end{figure}

\label{sec:Additional_Results}
\subsection{Visualization of Mask Position}
We visualized the mask of the $v$ matrix in the third attention layer of the second decoder block in the U-Net, as shown in Figure~\ref{fig:mask_position}. Although the mask ratio consistently remains at 8.24\%, its positions vary across different timesteps. This indicates that the mask introduces timestep dependency, allowing each timestep to have its unique U-Net weight distribution.
\begin{figure}[t]
  \centering
  % \fbox{\rule{0pt}{2in} \rule{0.9\linewidth}{0pt}}
   \includegraphics[width=1.\linewidth]{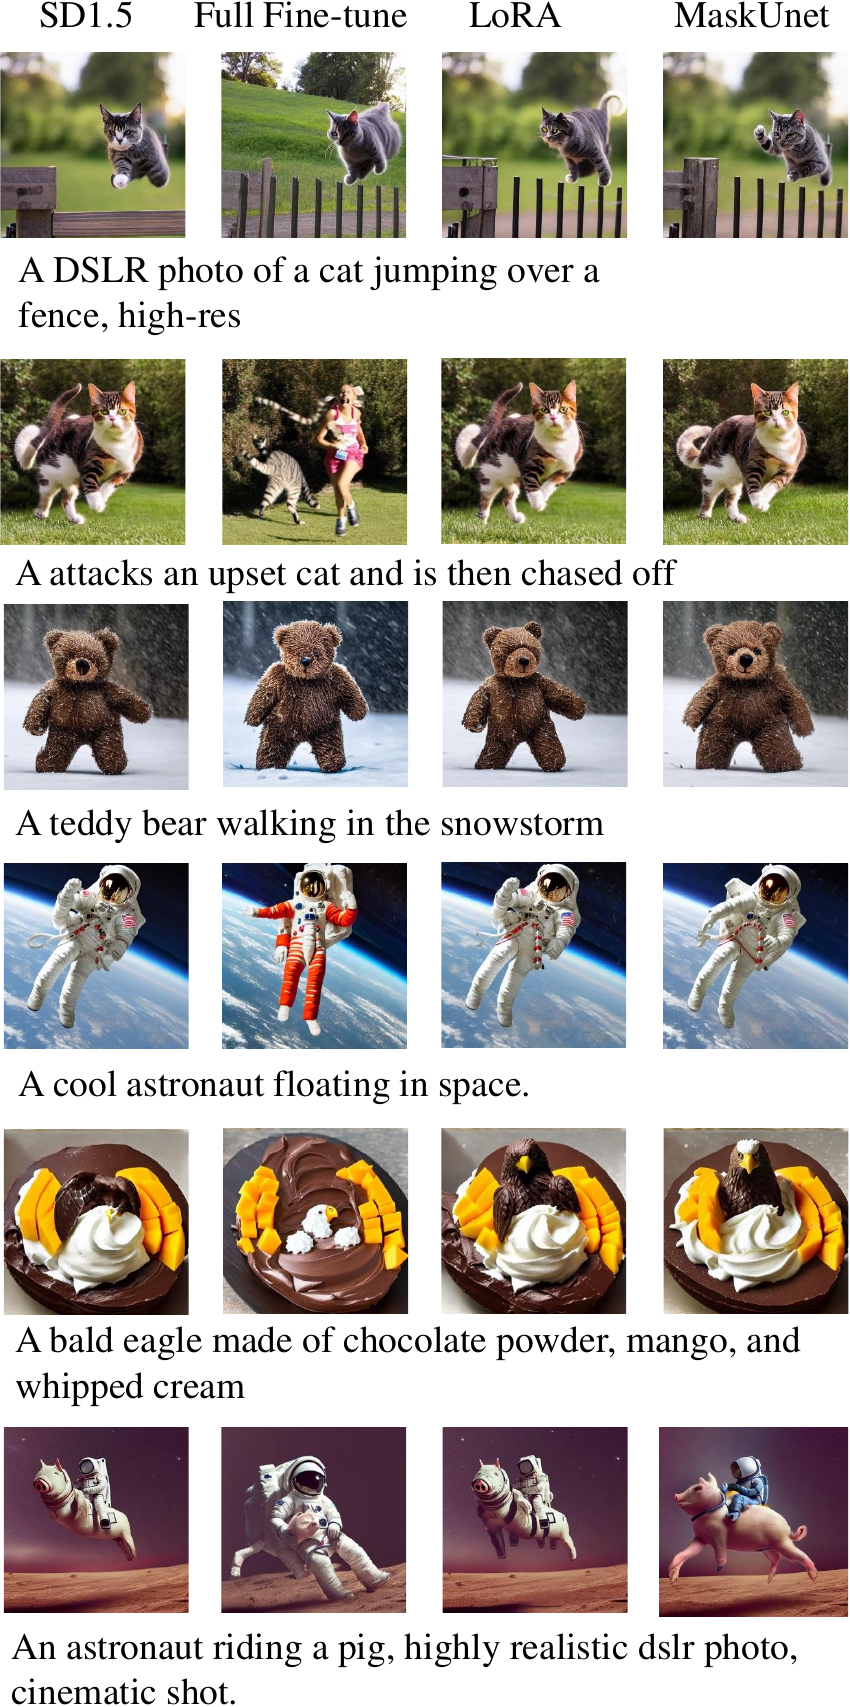}
   \vspace{-0.3cm}
   \caption{Quality results compared to other methods.}
   \label{fig:zero-shot-appendix}
% \vspace{-0.5cm}
\end{figure}
\begin{figure*}[t]
  \centering
  % \fbox{\rule{0pt}{2in} \rule{0.9\linewidth}{0pt}}
   \includegraphics[width=1.\linewidth]{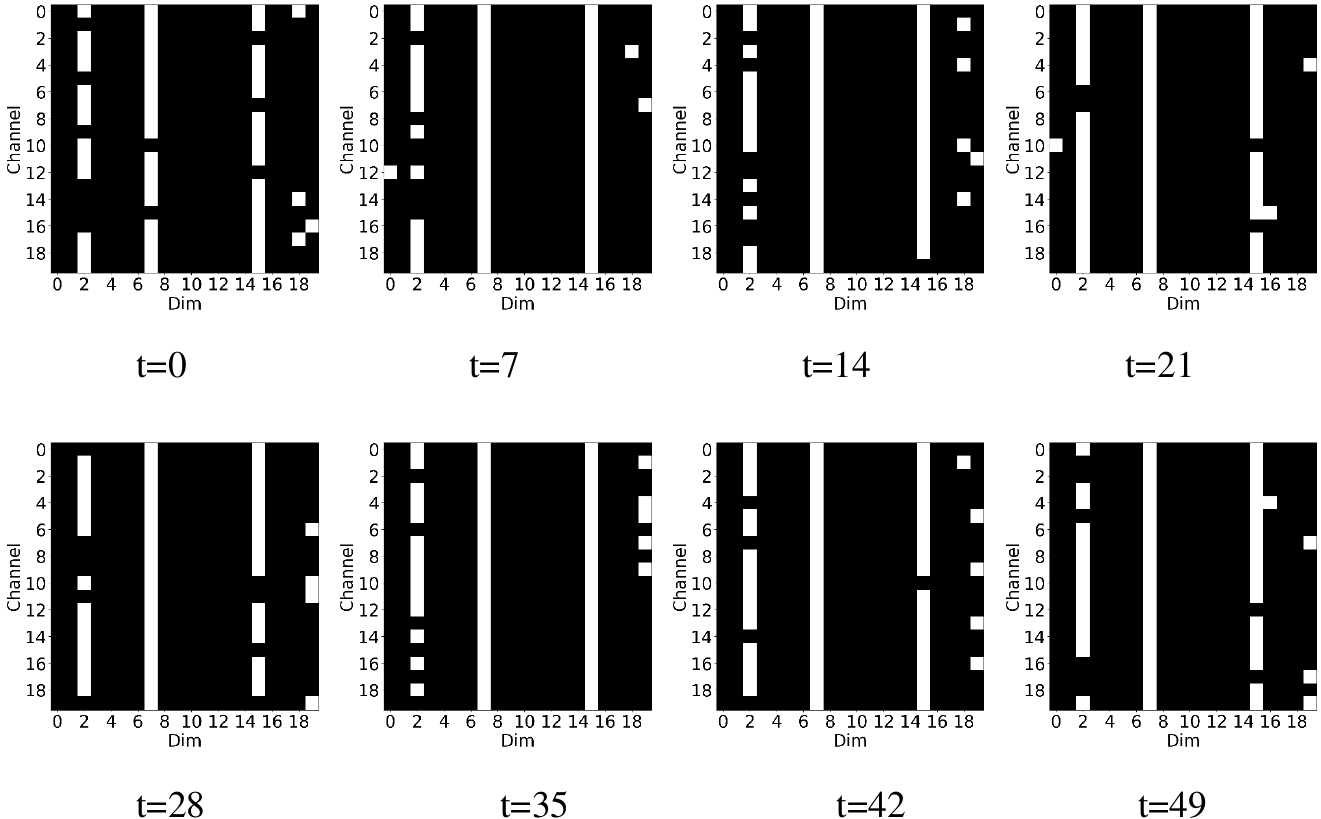}
   \vspace{-0.3cm}
   \caption{Visualization of mask position at different time steps.}
   \label{fig:mask_position}
% \vspace{-0.5cm}
\end{figure*}
\subsection{Text-to-video for More Visualization Results}
Additional visualization results of zero-shot generation are shown in the Figure~\ref{fig:zero-shot-appendix}. Figure~\ref{fig:text2video_com} is the complete visualization result of Text2Video-Zero~\cite{khachatryan2023text2video}. It clearly demonstrates that MaskUNet generates videos with greater temporal continuity and semantic consistency, validating its effectiveness in video generation.
\begin{figure*}[t]
  \centering
  % \fbox{\rule{0pt}{2in} \rule{0.9\linewidth}{0pt}}
   \includegraphics[width=1.\linewidth]{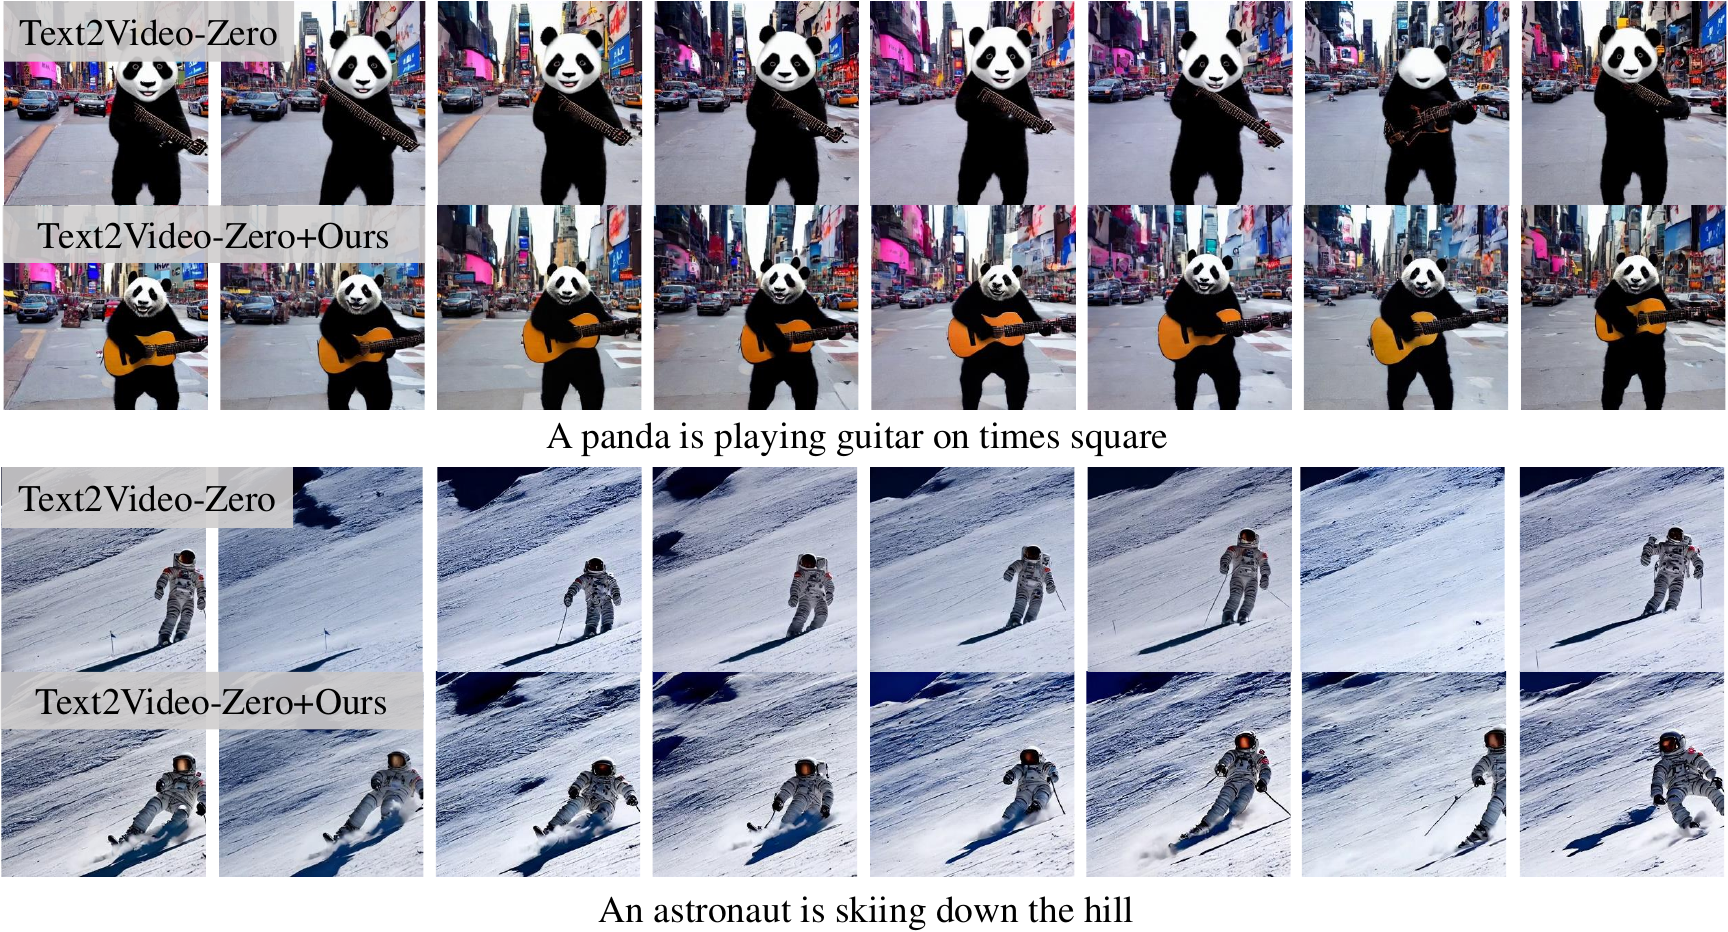}
   \vspace{-0.3cm}
   \caption{Quality results by Text2Video-Zero~\cite{khachatryan2023text2video} with or without mask.}
   \label{fig:text2video_com}
\vspace{-0.5cm}
\end{figure*}

\subsection{User study details}
The study participants consisted of 26 volunteers from our university. The questionnaire comprised 46 questions, each presenting several images: one generated by our method, MaskUNet, and the others generated by alternative methods (Dreambooth~\cite{ruiz2023dreambooth}, Textual Inversion~\cite{galimage}, Reversion~\cite{huang2023reversion}, Text2Video-zero~\cite{khachatryan2023text2video}, SynGen~\cite{rassin2024linguistic}, LoRA~\cite{hulora}, SD~\cite{rombach2022high}, etc.). An example of the questionnaire is shown in the Figure~\ref{fig:user_exam}.

% % 
% Having the supplementary compiled together with the main paper means that:
% % 
% \begin{itemize}
% \item The supplementary can back-reference sections of the main paper, for example, we can refer to \cref{sec:intro};
% \item The main paper can forward reference sub-sections within the supplementary explicitly (e.g. referring to a particular experiment); 
% \item When submitted to arXiv, the supplementary will already included at the end of the paper.
% \end{itemize}
% % 
% To split the supplementary pages from the main paper, you can use \href{https://support.apple.com/en-ca/guide/preview/prvw11793/mac#:~:text=Delete%20a%20page%20from%20a,or%20choose%20Edit%20%3E%20Delete).}{Preview (on macOS)}, \href{https://www.adobe.com/acrobat/how-to/delete-pages-from-pdf.html#:~:text=Choose%20%E2%80%9CTools%E2%80%9D%20%3E%20%E2%80%9COrganize,or%20pages%20from%20the%20file.}{Adobe Acrobat} (on all OSs), as well as \href{https://superuser.com/questions/517986/is-it-possible-to-delete-some-pages-of-a-pdf-document}{command line tools}.
